# Supplementary material for: A sharp-interface discontinuous Galerkin method for simulation of two-phase flow of real gases based on implicit shock tracking
Source: arXiv:2503.05557 source file (2025-03-07)
Supplement: Supplementary file 1 [file appendix_multiphase_roe_flux_prop.tex]

\section{Approximate Riemann Solver of Roe and Pike for multi-phase flow and non-ideal gas}
In this section we develop a Riemann solver for the two-phase Euler equations for two general convex equations of state. We follow the derivation developed by Roe and Pike \cite{roe1985efficient} in the case of an ideal gas, as well as that used by Glaister \cite{glaister1988approximate} for a non-ideal equation of state. 

Given two states $W_L$, $W_R$ of a gas close to an average state $W$, we seek coefficients $\alpha_j$ for all $j = 1, ..., m$ where $m$ is the number of equations, such that if $e_j$ are the eigenvectors of the Jacobian (\ref{eqn:evecs_multi}) matrix,
\begin{equation} \label{eqn:eigval_eqn_roeflux}
	\Delta W = \sum_{j = 1}^m \alpha_j e_j 
\end{equation}
where $\Delta (\cdot) = (\cdot)_R - (\cdot)_L$. For the $D = 1$ Euler equations, we have $m = 4$, and can solve \ref{eqn:eigval_eqn_roeflux} for the expressions
%\begin{equation}
	\begin{subequations}
		\begin{align}
			\alpha_1 &= \frac{1}{2c^2}(\Delta P + \rho c \Delta u) \\
			\alpha_2 &= \frac{1}{2c^2}(\Delta P - \rho c \Delta u) \\
			\alpha_3 &= \Delta \rho - \frac{\Delta P}{2c^2} \\
			\alpha_4 &= \Delta \rho + \frac{\Delta P}{2c^2} 
		\end{align}
	\end{subequations}
%\end{equation}

Next, we solve the algebraic problem for finding averages that hold exactly for arbitrary states $W_L$ and $W_R$ not necessarily close. We specifically seek averages $\hat{\rho}, \hat{u}, \hat{H}, \hat{\phi}, \hat{P_\rho},  \hat{P_e}$ and $\hat{P_{\rho \phi}}$ such that 
\begin{equation} \label{eqn:eigval_eqn_roeflux_averages}
	\Delta W = \sum_{j = 1}^m \hat{\alpha}_j \hat{e}_j 
\end{equation}
and 
\begin{equation} \label{eqn:flux_eqn_roeflux_averages}
	\Delta F = \sum_{j = 1}^m \hat{\lambda}_j \hat{\alpha}_j \hat{e}_j 
\end{equation}
where $\Delta (\cdot) = (\cdot)_R - (\cdot)_L$, $W$ and $F(W)$ are given from (\ref{eqn:multiphase_gov_eqn}). The averages for eigenvalues $\lambda_j$ and eigenvectors $e_j$ are given from (\ref{eqn:evals_multi}) and (\ref{eqn:evecs_multi}) as $\hat{\Lambda} = \Lambda(\hat{W}, N)$ and $\hat{W} = W(\hat{W}, N)$.
% Similarly, the speed of sound is given as  
%\begin{equation}
%\hat{c}^2 = \hat{P}_\rho + (\hat{H} - ||\hat{v}||^2) \frac{\hat{\bar{P}}_e}{\hat{\rho}} + \hat{\phi} \hat{P}_{\rho \phi}
%\end{equation}
and the expressions $\hat{\alpha}_j$ become 
\begin{subequations}\label{eqn:alpha_avg} 
		\begin{align}
			\hat{\alpha}_1 &= \frac{1}{2 \hat{c}^2}(\Delta P + \hat{\rho} \hat{c} \Delta u) \\
			\hat{\alpha}_2 &= \frac{1}{2\hat{c}^2}(\Delta P -\hat{ \rho} \hat{c} \Delta u) \\
			\hat{\alpha}_3 &= \Delta \rho - \frac{\Delta P}{2\hat{c}^2} \\
			\hat{\alpha}_4 &= \Delta \rho + \frac{\Delta P}{2\hat{c}^2} 
		\end{align}
\end{subequations}
and $\hat{c}$ is given by 
\begin{equation} \label{eqn:sndsp_roe_avg}
	\hat{\rho} \hat{c}^2  = \hat{\rho} \hat{P}_\rho \bigg|_{e, \rho \phi} + \hat{P}_e \bigg|_{\rho, \rho \phi}  \left(\frac{\hat{P}}{\hat{\rho}} \right) + \hat{\phi} \hat{\rho} \hat{P}_{\rho \phi}  \bigg|_{\rho, e} .
\end{equation}

We can begin by writing (\ref{eqn:eigval_eqn_roeflux_averages}) and (\ref{eqn:flux_eqn_roeflux_averages}) out explicitly
\begin{subequations}
	\label{eqn:roe_avg_all}
	\begin{align}
		\Delta \rho &= \hat{\alpha}_1 + \hat{\alpha}_2 + \hat{\alpha}_3 \label{eqn:roe_avg_eqn1} \\
		\Delta (\rho u) &= \hat{\alpha}_1 (\hat{v} + \hat{c}) + \hat{\alpha}_2 (\hat{v} - \hat{c}) + \hat{\alpha}_3 \hat{v} \label{eqn:roe_avg_eqn2} \\
		\Delta (\rho E) &= \hat{\alpha}_1 (\hat{H} + \hat{v} \hat{c}) + \hat{\alpha}_2 (\hat{H} - \hat{v} \hat{c}) + \hat{\alpha}_3 (\hat{v}^2 - \frac{\hat{P}_\rho \rho}{\hat{P}_e}) - \hat{\alpha}_4 \hat{P}_{\rho \phi} \label{eqn:roe_avg_eqn3} \\
		\Delta (\rho \phi) &= \hat{\alpha}_1 \hat{\phi} + \hat{\alpha}_2 \hat{\phi} - \hat{\alpha}_4 \frac{\hat{P}_e}{\hat{\rho}} \label{eqn:roe_avg_eqn4} \\
		\Delta (\rho u) &= \hat{\alpha}_1 (\hat{v} + \hat{c}) + \hat{\alpha}_2 (\hat{v} - \hat{c}) + \hat{\alpha}_3 \hat{v}  \label{eqn:roe_avg_eqn5}\\
		\Delta (P + \rho u^2) &= \Delta P + \Delta (\rho u^2) = \hat{\alpha}_1 (\hat{v} + \hat{c})^2 + \hat{\alpha}_2 (\hat{v} - \hat{c})^2 + \hat{\alpha}_3 \hat{v}^2 \label{eqn:roe_avg_eqn6}\\
		\Delta (u(\rho E + P)) &= \hat{\alpha}_1 (\hat{v} + \hat{c}) (\hat{H} + \hat{v} \hat{c}) + \hat{\alpha}_2 (\hat{v} - \hat{c}) (\hat{H} - \hat{v} \hat{c}) + \hat{\alpha}_3 \hat{u} (\hat{v}^2 - \frac{\hat{P}_\rho \rho}{\hat{P}_e}) - \hat{\alpha}_4 \hat{u} \hat{P}_{\rho \phi} \label{eqn:roe_avg_eqn7} \\
		 \Delta (\rho \phi u) &= \hat{\alpha}_1 (\hat{v} + \hat{c}) \hat{\phi} + \hat{\alpha}_2 (\hat{v} - \hat{c}) \hat{\phi} - \hat{\alpha}_4 \hat{v} \frac{\hat{P}_e}{\hat{\rho}} \label{eqn:roe_avg_eqn8} 
	\end{align}
\end{subequations}

{\color{red}{TO DO: finish derivation, from here, once $\alpha_j$ are known, it is straightforward to find averages}}

(\ref{eqn:roe_avg_eqn1})  is satisfied by any average we care to define and (\ref{eqn:roe_avg_eqn2}) is equivalent to (\ref{eqn:roe_avg_eqn5}). From this, we have from (\ref{eqn:roe_avg_eqn5}) 
\begin{equation} \label{eqn:roe_simp1}
	\begin{array}{c}
		\Delta (\rho u) =\hat{u} ( \hat{\alpha}_1 + \hat{\alpha}_2 + \hat{\alpha}_3) + \hat{c} ( \hat{\alpha}_1 - \hat{\alpha}_2) \\
		=\hat{u} \Delta \rho + \hat{\rho} \Delta u
	\end{array}
\end{equation}
and from (\ref{eqn:roe_avg_eqn6}) 
\begin{equation} \label{eqn:roe_simp2}
	\begin{array}{c}
		\Delta (\rho u^2) =\hat{u}^2 ( \hat{\alpha}_1 + \hat{\alpha}_2 + \hat{\alpha}_3) + 2 \hat{u} \hat{c} ( \hat{\alpha}_1 - \hat{\alpha}_2) \\
		=\hat{u}^2 \Delta \rho + 2 \hat{u} \hat{\rho} \Delta u.
	\end{array}
\end{equation}
Substituting for $\rho$ from (\ref{eqn:roe_simp1}) into (\ref{eqn:roe_simp2}) yields the quadratic equation for $\hat{u}$
\begin{equation}
	\hat{u} = \frac{\Delta(\rho u - \sqrt{(\Delta (\rho u) )^2 - \Delta \rho \Delta (\rho u^2 ) } }{ \Delta \rho}
\end{equation}
which yields the result 
\begin{equation} \label{eqn:u_avg}
	\hat{u} = \frac{ \sqrt{\rho_L} u_L + \sqrt{\rho_R} u_R}{\sqrt{\rho_L} + \sqrt{\rho_R} }.
\end{equation}
Substituting this into (\ref{eqn:roe_simp1}) gives 
\begin{equation} \label{eqn:rho_avg}
	\hat{\rho} = \frac{\Delta(\rho u) - \hat{u} \Delta \rho}{\Delta u} = \sqrt{ \rho_L \rho_R}
\end{equation}

We now show with (\ref{eqn:roe_avg_eqn3})  and (\ref{eqn:roe_avg_eqn7}) by rewriting them using (\ref{eqn:alpha_avg})  and (\ref{eqn:sndsp_roe_avg}) to obtain
\begin{equation} \label{eqn:roe_simp4}
	\Delta (\rho e) - \hat{e} \Delta \rho - \frac{\hat{\rho} \Delta P}{\hat{\rho} \hat{c}^2} + \hat{\alpha}_3 \hat{\rho} \frac{\hat{P}_\rho}{\hat{P}_e}
\end{equation}
and 
\begin{equation} \label{eqn:roe_simp5}
\begin{array}{c}
	0 =\Delta(\rho u e) - \hat{u} \hat{e} \Delta \rho - \hat{\rho} \hat{e} \Delta u + \Delta (u P) - \hat{u} \Delta P - \hat{P} \Delta u  + \Delta \left( \frac{\rho}{2} \hat{u}^3 \right) - \frac{u^3}{2} \Delta \rho - \frac{3}{2} \hat{\rho} \hat{u}^2 \Delta u \\ - \frac{\hat{u} \hat{P} \Delta \rho}{\hat{\rho}\hat{c}^2} + \hat{\alpha}_3 \hat{u} \hat{\rho} \frac{\hat{P}_\rho }{\hat{P}_e}
\end{array}
\end{equation}

Now from manipulation of expressions for $\hat{\rho}$ (\ref{eqn:rho_avg}) and $\hat{u}$ (\ref{eqn:u_avg}) along with (\ref{eqn:roe_simp4}) and (\ref{eqn:roe_simp5}) we can obtain 
\begin{equation}
	\frac{\hat{P}}{\hat{\rho}} + \hat{e} + \frac{1}{2} \hat{u}^2 = \frac{ \left( \sqrt{\rho_L} \left( \frac{P_L}{\rho_L} + e_L + \frac{1}{2} u^2_L \right) + \sqrt{\rho_R} \left( \frac{P_R}{\rho_R} + e_R + \frac{1}{2} u^2_R \right) \right) } {\left( \sqrt{\rho_L} + \sqrt{\rho_R}\right) }
\end{equation}
and defining a mean enthalpy $\hat{H}$ as 
\begin{equation}
\hat{H} = \frac{\hat{P}}{\hat{\rho}} + \hat{e} + \frac{1}{2} \hat{u}^2
\end{equation}
we find 
\begin{equation}
	\hat{H} = \frac{ \sqrt{\rho_L} H_L + \sqrt{\rho_R} H_R } {\sqrt{\rho_L} + \sqrt{\rho_R}}
\end{equation}
which is similar to that of the ideal gas case. 

\new{write out for $\hat{\phi}$ }

Now we have specified $\hat{\rho}$, $\hat{u}$, and $\hat{H}$, we focus on specifying $\hat{P}_\rho$, $\hat{P}_e$, and $\hat{P}_{\rho \phi}$. We now focus our attention on (\ref{eqn:roe_simp4}) which can be simplified to obtain 
\begin{equation}
	\Delta (\rho e) - \hat{e} \Delta \rho - \hat{\rho} \Delta e + \frac{\hat{\rho}}{\hat{P}_e} \left( \hat{P}_e \Delta e + \hat{P}_\rho \Delta \rho + \hat{P}_{\rho \phi} \Delta (\rho \phi) - \Delta P \right) = 0
\end{equation}
We make the natural choice of 
\begin{equation}
	\Delta (\rho e) - \hat{e} \Delta \rho - \hat{\rho} \Delta e = 0
\end{equation}
whic leads to 
\begin{equation}  \label{eqn:u_avg}
	\hat{e} = \frac{ \sqrt{\rho_L} e_L + \sqrt{\rho_R} e_R}{\sqrt{\rho_L} + \sqrt{\rho_R} }.
\end{equation}
This leads to the relation
\begin{equation} \label{eqn:roe_avg_press_relation}
	\Delta P = \hat{P}_\rho \Delta \rho + \hat{P}_e \Delta e + \hat{P}_{\rho \phi} \Delta (\rho \phi)
\end{equation}
as a necessary condition. From this, to complete the approximate Riemann solver we must choose approximations for the averages $\hat{P}_\rho$, $\hat{P}_e$, and $\hat{P}_{\rho \phi}$ to $P_\rho$, $P_e$, and $P_{\rho \phi}$ respectively so that (\ref{eqn:roe_avg_press_relation}) holds. We find thes approximations as 

\begin{equation}
	\text{something}
\end{equation}

In practice, we must numerically check that the differences $\Delta \rho$, $\Delta e$, and $\Delta (\rho \phi)$ are near zero. This is a delicate matter, especially as there can be large magnitude difference in the state variables. For example, $\Delta e$ may be on a magnitude of $\approx \mathcal{O}(10^5)$ while $\Delta (\rho \phi)$  has a difference on order  $\approx \mathcal{O}(1)$. Therefor we introduce a check based on the normalized difference between the two states, 
\begin{equation}
	\text{something}
\end{equation}
